# Supplementary material for: Stress anisotropy in confined populations of growing rods
Source: arXiv:2207.02607 ancillary file (2022-07-06)
Supplement: Supplementary file 1 [file supplement.pdf]

# Supplementary Information: Stress anisotropy in confined populations of growing rods

Jonas Isensee, Lukas Hupe, Ramin Golestanian, and Philip Bittihn

## 1 Model Definition

In this section, we discuss the details of our agent-based model of dividing rod-shaped bacteria. Many aspects of the model are shared with models commonly used in literature [1, 2, 3, 4, 5, 6].

We model bacteria as two-dimensional spherocylinders of radius $R$ around the backbone, a line segment of length $b_i$ and orientation $\varphi_i$ extending symmetrically from the centre of mass position $\mathbf{r}_i^{\mathrm{cm}}$, as illustrated in Fig. 1A. Thus, the total end-to-end length $l_i$ of a cell is equal to $b_i + 2R$ and its width is $2R$. The backbone length $b_i$ is governed by an internal spring of rest length $b^{\mathrm{eq}}$.

To model the cellular life cycle, every cell has an internal clock $g_i \in [0, 1)$ which advances linearly in time with a growth rate $\gamma_i$. Growth is modelled implicitly, by changing the rest length of the internal spring

$$b^{\mathrm{eq}}(g_i, l_{\max}, R) = \frac{l_{\max}}{2} \cdot (g_i + 1) - 2R\,. \tag{1}$$

At $g_i = 1$, the cell reaches its division length $l_{\max}$ and is divided into two equally sized children, each initialised with internal clocks set to zero. The growth rates of these children are drawn independently from the growth rate distribution $P(\gamma)$ to desynchronise the division events. Here, we choose equidistributed growth rates from an interval $[0.75, 1.25]$.

### 1.1 Equations of motion

Using overdamped dynamics, we write the equations of motion as

$$\frac{\mathrm{d}}{\mathrm{d}t}\mathbf{r}_i^{\mathrm{cm}} = \mu^{\mathrm{cm}}(b_i, \varphi_i) \cdot \mathbf{F}_i^{\mathrm{cm}} \tag{2}$$

$$\frac{\mathrm{d}}{\mathrm{d}t} b_i = \mu^{\mathrm{int}}(b_i) \cdot F_i^{\mathrm{int}} \tag{3}$$

$$\frac{\mathrm{d}}{\mathrm{d}t}\varphi_i = \mu^{\mathrm{rot}}(b_i) \cdot T_i. \tag{4}$$

where $\mu^{\mathrm{cm}}$ is the translational mobility tensor, $\mu^{\mathrm{int}}$ and $\mu^{\mathrm{rot}}$ are the mobilities of the internal and rotation degree of freedom respectively, $\mathbf{F}_i^{\mathrm{cm}}$ is the force acting

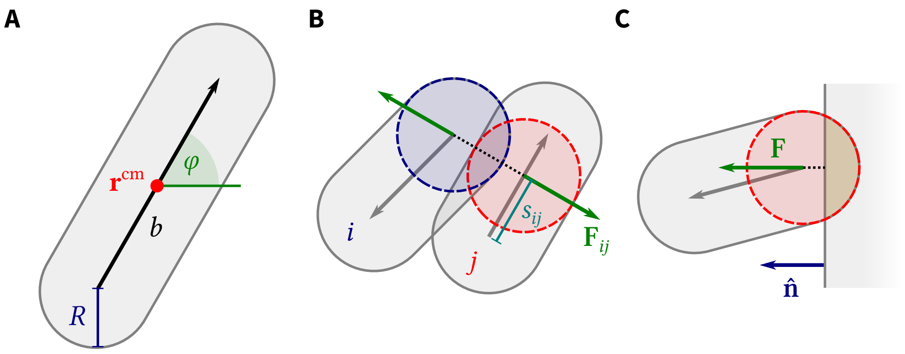


**Figure 1:** **a** Illustration of a single rod-shaped cell, with backbone of length $b$, orientation $\varphi$, centre of mass position $\mathbf{r}^{\rm cm}$ and radius $R$. **b** Interaction between two cells $i$ and $j$, with virtual Hertzian nodes, interaction force $\mathbf{F}_{ij}$ and projected attack point $s_{ij}$. **c** Interaction between a cell and a straight wall, with a virtual Hertzian node and interaction force.

on its centre of mass, $F_i^{\rm int}$ is the force acting on the internal degree of freedom and $T_i$ is the torque with respect to the centre of mass.

Assuming that $\mu^{\rm cm}$ is diagonal in the reference frame of the backbone, we decompose the right-hand side of Eq. (2) into parallel and perpendicular components with respect to the backbone.

$$\frac{\mathrm{d}}{\mathrm{d}t}\mathbf{r}_i^{\rm cm} = \mu^{\parallel}(b_i)\, F_i^{\parallel} \cdot \hat{\mathbf{e}}_i + \mu^{\perp}(b_i)\, F_i^{\perp} \cdot (\hat{\mathbf{z}} \times \hat{\mathbf{e}}_i) \tag{5}$$

where $\hat{\mathbf{e}}_i = (\cos(\varphi_i), \sin(\varphi_i))^{\rm T}$ and the two-dimensional "cross product" is defined as $\hat{\mathbf{z}} \times (x_1, x_2)^{\rm T} = (-x_2, x_1)^{\rm T}$.

We then use a numerical approximation for the mobilities of rods in a viscous fluid, derived by Tirado et al. [7, 8, 9, 10], to set the external mobilities $\mu^{\parallel}$, $\mu^{\perp}$ and $\mu^{\rm rot}$ to

$$\mu^{\parallel}(a) = \frac{1}{2\pi\,\eta\,(2R\,a)}\left(\log(a) - 0.207 + 0.980\,a^{-1} - 0.133\,a^{-2}\right) \tag{6}$$

$$\mu^{\perp}(a) = \frac{1}{4\pi\,\eta\,(2R\,a)}\left(\log(a) + 0.839 + 0.185\,a^{-1} + 0.233\,a^{-2}\right) \tag{7}$$

$$\mu^{\rm rot}(a) = \frac{3}{\pi\,\eta\,(2R\,a)^3}\left(\log(a) - 0.662 + 0.917\,a^{-1} - 0.050\,a^{-2}\right) \tag{8}$$

where $a = b_i/2R + 1$ is the aspect ratio of the cell. These expressions are valid approximations for rod-shaped objects with aspect ratios in the range of $2 < a < 30$ [7].

We choose the internal mobility $\mu^{\rm int}$ to be equal to $2\mu^{\parallel}$ to ensure that the internal degree of freedom does not relax faster than the centre of mass movement. This choice prevents inconsistent behaviour, as can be demonstrated with

a simple example: If a force parallel to the backbone is applied to one end of a cell only, the motion of the other side of the cell depends on the ratio between the internal and external mobilities. If the internal degree of freedom relaxes faster than the centre of mass, this could cause the other end of the cell to move against the direction of the force.

## 1.2 Interactions

In this model, forces arise from two processes:

- pairwise steric interactions between particles
- compression of the internal spring acting on the backbone length

The force $\mathbf{F}_{ij}$ exerted on cell $j$ by its interaction with cell $i$ is modelled as a function of the shortest distance vector $\mathbf{d}_{ij}$ between their backbones, with

$$\mathbf{F}_{ij}(\mathbf{d}_{ij}) = \begin{cases} \frac{Y}{2}\sqrt{\frac{R}{2}}\left(2R - \|\mathbf{d}_{ij}\|\right)^{3/2} \cdot \frac{\mathbf{d}_{ij}}{\|\mathbf{d}_{ij}\|} & \|\mathbf{d}_{ij}\| \leq 2R \\ 0 & \|\mathbf{d}_{ij}\| > 2R \end{cases} . \tag{9}$$

This Hertzian potential is equivalent to the contact forces of two virtual elastic disks of Young's modulus $Y$[1], positioned on the cell backbones at the points of closest approach, as illustrated in Figure 1B. It should be noted that by this construction, forces can only act orthogonally to the cell boundary.

We now need to decompose $\mathbf{F}_{ij}$ into the force components used in the equations of motion for cell $j$. The total force determines the centre of mass movement, i.e.

$$\mathbf{F}_{ij}^{\mathrm{cm}} = \mathbf{F}_{ij}. \tag{10}$$

To compute the contributions to the torque and internal force, we project the attack point $\mathbf{r}_{ij}$ of $\mathbf{F}_{ij}$ on cell $j$'s backbone, i.e.

$$\max\left(\min\left(\frac{\left(\mathbf{r}_{ij}^{\mathrm{F}} - \mathbf{r}_i^-\right) \cdot \hat{\mathbf{e}}_j}{b_j}, 1\right), 0\right) =: s_{ij} \in [0, 1] \tag{11}$$

where $b_j$ is the length of the backbone. We can now write the torque $T_{ij}$ with respect to the centre of mass as

$$T_{ij} = b_j \frac{1 - 2s_{ij}}{2} \hat{\mathbf{e}}_j \times \mathbf{F}_{ij} \tag{12}$$

and the contribution to the internal force as

$$F_{ij}^{\mathrm{int}} = \hat{\mathbf{e}}_j \cdot \mathbf{F}_{ij} \cdot \begin{cases} 1 & \text{if } s_{ij} = 0 \\ -1 & \text{if } s_{ij} = 1 \\ 0 & \text{else} \end{cases} , \tag{13}$$

[1]Technically, this is the effective elastic modulus $Y^*$, which also contains the Poisson's ratio of the materials (definition in [11, Eq. (2.1)])

since by construction, only forces attacking at the semicircular caps can compress the internal spring.

To counteract external compression of the backbone, we compute a restoring force using the same Hertzian force law for simplicity

$$\mathbf{F}_j^{\mathrm{int}} = \frac{Y}{2}\sqrt{\frac{R}{2}} \cdot \mathrm{sgn}(\Delta b_j) \cdot |\Delta b_j|^{3/2}\, \hat{\mathbf{e}}_j \,, \tag{14}$$

with $\Delta b_j = b^{\mathrm{eq}}(g_j, l_{\mathrm{max}}) - b_j$.

## 1.3 Domain boundaries

In this paper, non-periodic systems can have two types of domain boundaries

- *Open boundaries.* When a cell's centre of mass crosses an open or absorbing boundary, it is removed from the system. This corresponds to a force-free boundary in the continuum picture. Here, every system must contain at least one open boundary to reach a steady state: since growth constantly creates new cells, removal is necessary to keep the cell number constant.
- *Walls.* Solid walls exert a repulsive force on cells and correspond to a zero-velocity boundary in the continuum description. Note that, due to the anisotropic shape of the cells, walls will in most cases also create local parallel alignment.

Since all cell-cell interactions are modelled as Hertzian spheres, we decided to use a similar approach to model the interactions with confining walls, slightly modified to account for the fact that the wall has zero curvature. The force due to interaction with a wall is thus

$$\mathbf{F}(d) = \left(\frac{1}{Y} + \frac{1}{Y^{\mathrm{w}}}\right)^{-1} \sqrt{R}(R-d)^{3/2}\, \hat{\mathbf{n}} \,, \tag{15}$$

where $d$ is the closest distance of the cell backbone to the wall, $\hat{\mathbf{n}}$ is the wall normal and $Y^{\mathrm{w}}$ is the wall hardness (compare Fig. 1c). Assuming that walls are generally much harder than bacteria, we let $Y^{\mathrm{w}} \longrightarrow \infty$, thus simplifying the hardness prefactor of the force law to $Y$.

## Setup and Procedures for Simulations

A simulation is set up by placing four rods into the centre of the domain where orientation and cell growth progress are drawn independently from a uniform distribution. Time integration is realized using an Euler integrator with adaptive step sizes to limit the maximal displacement of cells. Snapshots are stored at regular intervals such that there are ten snapshots for every cell generation. All model parameters kept unchanged for all simulations in this work are given in Table 2 and all further settings in Table 1.

| domain width | boundary | division length $l_{\max}$ | ics | time | discarded transient |
|---|---|---|---|---|---|
| 200 | walls | 2, 2.25, ..., 6 | 10 | 30 | 25 |
| 200, 200.1, ..., 205 | walls | 6 | 20 | 40 | 25 |
| 1dim | - | 2, 2.25, ..., 6 | 25 | 110 | 10 |
| 600 | open | 2, 2.25, ..., 6 | 10 | 30 | 25 |
| 600 | open | 6 | 200 | 40 | 25 |

**Table 1:** Simulations sets

| | |
|---|---|
| cell diameter $2R$ | 1 |
| domain height | 200 |
| viscosity $\eta$ | 0.05 |
| Young's modulusY | 1.6e6 |
| growthrate distr | $\mathcal{U}_{[0.75,1.25]}$ |

**Table 2:** Model parameters identical in all simulations.

# 2 1D Continuum model

## 2.1 Population Demographics

The full description of the agent-based model depends on many aspects such as the domain geometry and the resulting flow. To simplify the picture, we will for now forget about the spatial dynamics. The only relevant aspect in the following considerations is that cells age according to their growth rate $\gamma$ drawn from the uniform distribution

$$G(\gamma) = \begin{cases} \frac{1}{\Delta\gamma}, & \gamma_0 - \frac{\Delta\gamma}{2} \leq \gamma \leq \gamma_0 + \frac{\Delta\gamma}{2} \\ 0, & \text{else} \end{cases}$$

at cell birth and divide when their growth progress reaches $g = 1$.

The first step in this theoretical description is to consider the probability $p(g, \gamma, t)$ for any cell in a colony to have growth rate $\gamma$ and be at growth progress $g$. The distribution for an exponentially growing colony must solve the equation

$$\frac{\partial p}{\partial t} = -\gamma \frac{\partial p}{\partial g} - p \int \gamma' p(1, \gamma', t) \, \mathrm{d}\gamma' \tag{16}$$

where the first term accounts for the ageing of cells and the second term corresponds to random cell removal to keep the distribution normalized. The form of said term can best be explained by comparison with the boundary condition of cell division

$$\int \gamma p(0, \gamma, t) \, \mathrm{d}\gamma = 2 \int \gamma p(1, \gamma, t) \, \mathrm{d}\gamma$$

which is a continuum version of stating that every cell divides into two daughter cells with $g = 0$. The additional $\gamma$ in the integrands are needed to properly

scale time and naturally turn up when deriving the above equation as a limit of divisions within a small time interval. This boundary condition, together with the advective first term of Eq. (16), models the population dynamics observed in the agent based simulations.

## 2.2 Steady State Solution

In the following, we will mostly be concerned with the steady-state dynamics of the growing colony. For this case, we can write down an analytical solution of Eq. (16)

$$p(g,\gamma) = \frac{\chi}{\gamma} G(\gamma) \exp\left(-\frac{\chi}{2\gamma} g\right) \tag{17}$$

which can be found by defining

$$\chi(t) = 2 \int \gamma p(1,\gamma,t)\,\mathrm{d}\gamma \tag{18}$$

and setting the time derivative in Eq. (16) to zero, which gives the linear differential equation solved by Eq. (17)

$$\frac{\partial p}{\partial g} = -\frac{\chi}{2\gamma} p.$$

To accurately compute the (steady-state) normalization $\chi$ we plug Eq. (17) into Eq. (18) and obtain

$$\begin{aligned}
\chi &= 2 \int \gamma \left( \frac{\chi}{\gamma} G(\gamma) \exp\left\{-\frac{\chi}{2\gamma}\right\}\right) \mathrm{d}\gamma \\
&= 2\chi \int G(\gamma) \exp\left\{-\frac{\chi}{2\gamma}\right\} \mathrm{d}\gamma \\
&= \frac{2\chi}{\Delta\gamma} \left[ \frac{\chi}{2} \mathbf{Ei}\left(\frac{-\chi}{2\gamma}\right) + \gamma \exp\left\{-\frac{\chi}{2\gamma}\right\}\right]_{\gamma_0-\Delta\gamma/2}^{\gamma_0+\Delta\gamma/2} \\
\Rightarrow 0 &= -1 + \frac{2}{\Delta\gamma} \left[ \frac{\chi}{2} \mathbf{Ei}\left(-\frac{\chi}{2\gamma}\right) + \gamma \exp\left\{-\frac{\chi}{2\gamma}\right\}\right]_{\gamma_0-\Delta\gamma/2}^{\gamma_0+\Delta\gamma/2}
\end{aligned}$$

with **Ei** the exponential integral and where the last expression can be solved for $\chi$ using numerical root finding. All simulations in this work assume a growth rate distribution where the width $\Delta\gamma = \gamma_0/2$ is half of the mean value and for these parameters we obtain

$$\begin{aligned}
\langle \gamma \rangle &\approx 0.985\,\gamma_0 \\
\langle g \rangle &\approx 0.441
\end{aligned} \tag{19}$$

which is independent of all other system parameters.

To bridge the gap to agent-based simulations, we need to discuss what the assumptions underlying the continuum theory say about the channel simulations. An agent-based simulation of rods in a channel geometry has an approximately constant number of rods in the steady-state. This is achieved by removal of all cells that are pushed out of the domain. The continuum theory on the other hand, has no notion of space and removes cells uniformly by a continuous rescaling term. For these two processes to be equivalent, the distribution of growth progress $g$ and growth rate $\gamma$ in the simulations must be *well-mixed*.

The randomization of growth rates at cell division ensures such a constant mixing of the population structure in the agent-based simulations. Due to this and due to the indiscriminate removal of cells at the boundary, it turns out that the distribution of cells in the confined domains are well approximated by these equations, as can be seen in Fig. 2. There, spatially resolved estimates for $\langle\gamma\rangle$ and $\langle g\rangle$ are drawn alongside the predictions from Eq. (19) and it can be seen that relative deviations from the expected averages are small. Special care

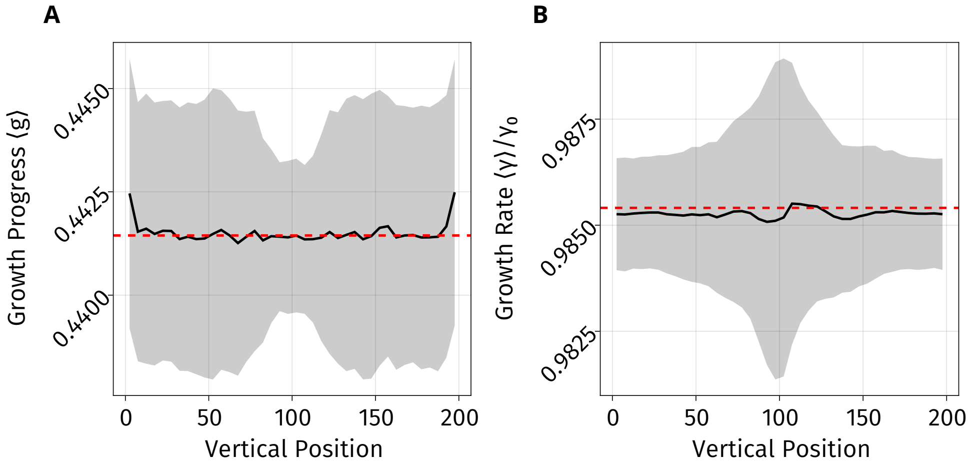


**Figure 2:** Numerical estimates for the averages $\langle g\rangle$ in pane A and $\langle\gamma\rangle$ in B from simulations on 200 unit tall domains with temporal and ensemble averaging using $l_{\max} = 6$. Shaded regions indicate the standard deviation of fluctuations.

needs to be taken when computing the averages in a spatially resolved manner as Eq. (17) pertains to the number distribution while in the actual simulations larger cells cover more area and estimates might introduce a bias based on that. For this reason we employed a simpler binning approach in combination with a low spatial resolution.

Having convinced ourselves that the distribution in Eq. (17) indeed models the population demographics of the agent-based simulations accurately, we can build upon this and move on to derive further predictions.

## 2.3 Defining Units

The model studied in this paper contains many different parameters and yields rich dynamics. This makes it important to define useful units to allow for meaningful comparisons between results of different parameters. The first and simplest unit to define is length, as all growing rods in our model share the same fixed width equal to 1.

Due to the linear nature of the overdamped dynamics, a physical time can only be defined in relation to both numerical growth rate and viscosity and is ambiguous under proportional scaling of these parameters. As a result, we set the reference growth rate as unity and use in all figures displaying time evolution the cumulative generation time as the abscissa.

At the core of this work lie measurements of the stress tensor. Within confinement, stresses arise from configuration-dependent mechanical interactions. However, as discussed above, even along the unconfined axis inside channels there is a well-defined stress field due to surface friction of the expansion flow. We will, thus, use the in-compressible theory derived in the main text to define a unit stress as

$$S_0 = \left\langle \mu_{||}^{-1} \right\rangle \frac{\langle \gamma \rangle \, 10^4}{2\langle 1+g \rangle^2}$$

which is the (hypothetical) central stress of a $y_{\max} = 100$ domain with the longest rods $l_{\max} = 6$ used and all other parameter taken from Table 2.

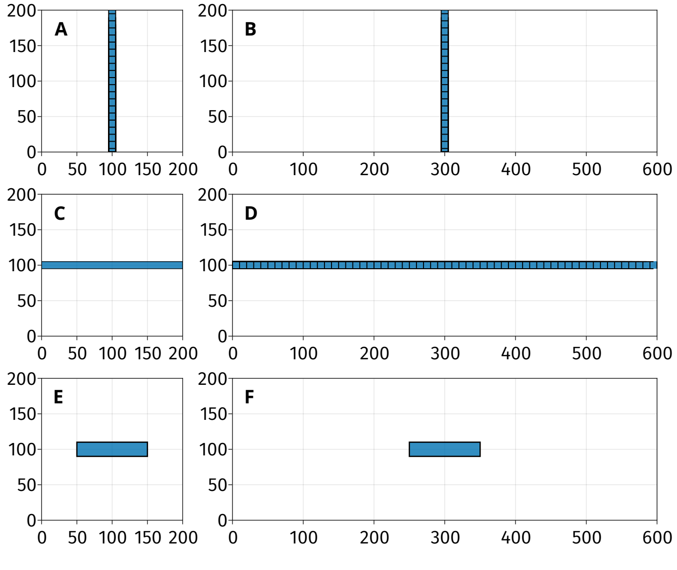


**Figure 3:** Illustration of regions used to estimate stress tensor field values. (a) used in Fig. 1 (b) used in Fig. 4 (c) used in Fig. 3 (full width) (d) used in Fig. 4 (e) used in Fig. 5 (f) used in Fig. 5

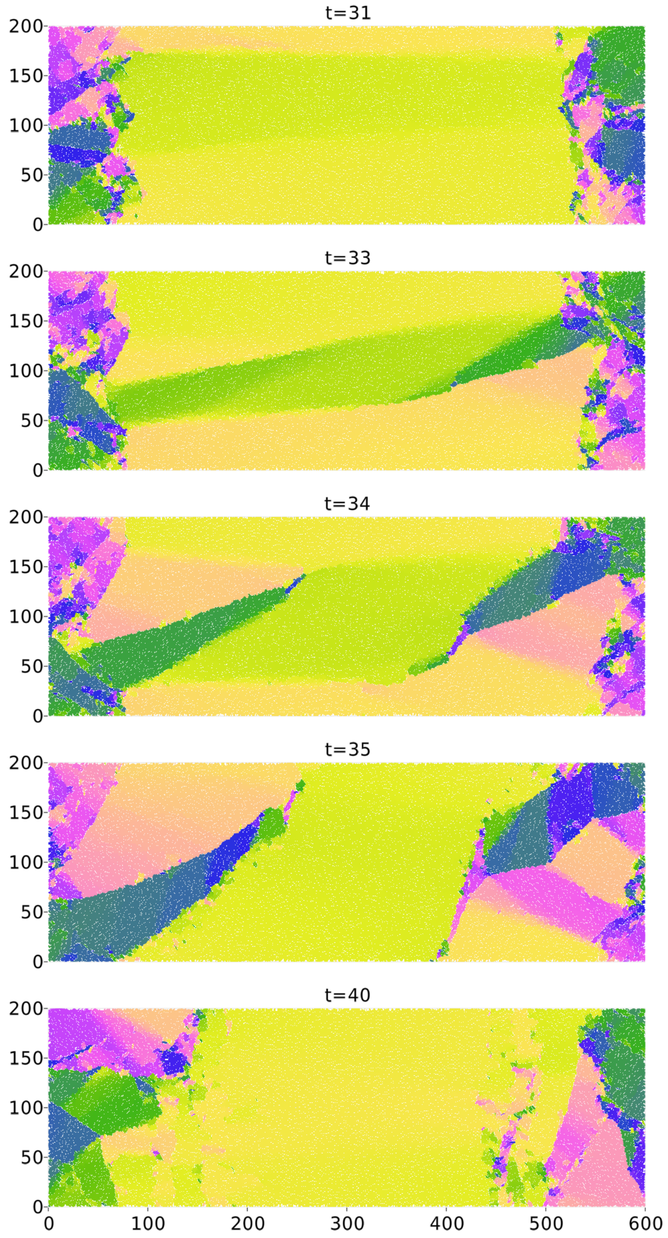


**Figure 4:** Example of macroscopic buckling even and subsequent relaxation to order. Shown are snapshots at different times of an open-domain simulation using $l_{\max} = 6$ rods.

# References


[1] Duco van Holthe tot Echten, Gerhard Nordemann, Martijn Wehrens, Sander Tans, and Timon Idema. Defect dynamics in growing bacterial colonies. *arXiv*, page 2003.10509, 2020.

[2] Tomas Storck, Cristian Picioreanu, Bernardino Virdis, and Damien J. Batstone. Variable Cell Morphology Approach for Individual-Based Modeling of Microbial Communities. *Biophysical Journal*, 106(9):2037–2048, 2014.

[3] Sirio Orozco-Fuentes and Denis Boyer. Order, intermittency, and pressure fluctuations in a system of proliferating rods. *Phys. Rev. E*, 88(1):012715, 2013.

[4] Dmitri Volfson, Scott Cookson, Jeff Hasty, and Lev S. Tsimring. Biomechanical ordering of dense cell populations. *PNAS*, 105(40):15346–15351, 2008.

[5] HoJung Cho, Ann M Stevens, Alex Groisman, and Andre Levchenko. Self-Organization in High-Density Bacterial Colonies: Efficient Crowd Control. *PLoS Biology*, 5(11):10, 2007.

[6] Zhihong You, Daniel J. G. Pearce, Anupam Sengupta, and Luca Giomi. Geometry and Mechanics of Microdomains in Growing Bacterial Colonies. *Phys. Rev. X*, 8(3):031065, 2018.

[7] M. Mercedes Tirado, Carmen López Martínez, and José García de la Torre. Comparison of theories for the translational and rotational diffusion coefficients of rod-like macromolecules. Application to short DNA fragments. *J. Chem. Phys.*, 81(4):2047–2052, 1984.

[8] Maria M. Tirado and José García de la Torre. Translational friction coefficients of rigid, symmetric top macromolecules. Application to circular cylinders. *J. Chem. Phys.*, 71(6):2581–2587, 1979.

[9] María M. Tirado and José García de la Torre. Rotational dynamics of rigid, symmetric top macromolecules. Application to circular cylinders. *J. Chem. Phys.*, 73(4):1986–1993, 1980.

[10] Henricus H. Wensink, Jörn Dunkel, Sebastian Heidenreich, Knut Drescher, Raymond E. Goldstein, Hartmut Löwen, and Julia M. Yeomans. Meso-scale turbulence in living fluids. *PNAS*, 109(36):14308–14313, 2012.

[11] Emanuel Willert, Markus Heß, and Valentin L Popov. *Handbook of Contact Mechanics.* 2019.
